# Supplementary material for: TSAQA: Time Series Analysis Question And Answering Benchmark
Source: arXiv:2601.23204 source file (2026-06-05)
Supplement: Supplementary file 1 [file 11_appendix_statements.tex]

\newpage
\section{The Use of Large Language Models}
